# Supplementary material for: P-graph Associahedra and Hypercube Graph Associahedra
Source: arXiv:2211.02113 source file (2022-11-03)
Supplement: Supplementary file 1 [file Appendix-B.tex]

\chapter{Variables}

A summary of all variables is documented in Table \ref{tab:vars}.

\begin{longtable}{| l | l |}
\caption{A summary of common meteorological variables and their abbreviations in alphabetical order.}\label{tab:vars}\\
\hline 
Variable & Abbreviation \\
\hline
Arbitrary variable & $X$ \\
Absolute vorticity vector & $\vec{\eta}$ \\
Coriolis parameter & $f$ \\
Gas constant for dry air & $R$ \\
Geopotential & $\Phi$ \\
Geopotential height & $Z$ \\
Gravitational accelleration & $g$ \\
Horizontal wind vector & $\vec{V}$ \\
Isobaric vertical motion & $\omega$ \\
Latent heat of vaporization & $l_v$ \\
Meridional unit vector & $\hat{j}$ \\
Meridional wind & $v$ \\
Potential temperature & $\theta$ \\
Potential vorticity & $P$ \\
Pressure & $p$ \\
Relative vorticity vector & $\vec{\zeta}$  \\
Specific density & $\alpha$ \\
Specific heat capacity at constant pressure & $c_p$ \\
Temperature & $T$ \\
Time & $t$ \\
Three-dimensional wind vector & $\vec{U}$ \\
Vertical absolute vorticity & $\eta$ \\
Vertical unit vector & $\hat{k}$ \\
Vertical relative vorticity & $\zeta$ \\
Zonal unit vector & $\hat{i}$ \\
Zonal wind & $u$ \\
\hline
\end{longtable}
